# Supplementary material for: Electric Current Control of Helimagnetic Chirality from a Multidomain State in the Helimagnet MnAu$_2$
Source: arXiv:2511.22032 source file (2026-06-10)
Supplement: Supplementary file 1 [file SupplementalMaterial.tex]

% For Phys. Rev. appearance, change preprint to twocolumn.
% Choose pra, prb, prc, prd, pre, prl, prstab, or rmp for journal
%  Add 'draft' option to mark overfull boxes with black boxes
%  Add 'showpacs' option to make PACS codes appear
%  Add 'showkeys' option to make keywords appear
%\documentclass[aps,prl,preprint,groupedaddress]{revtex4}
%\documentclass[aps,prl,twocolumn,superscriptaddress,showpacs,longbibliography]{revtex4} % for PRX
%\documentclass[aps,prl,twocolumn,superscriptaddress,showpacs]{revtex4} % for PRL
\documentclass[preprint,aps,
% prl,
superscriptaddress,onecolumn,amsmath,amssymb,nofootinbib,nobibnotes]{revtex4-2} % for PRL
%\documentclass[aps,prl,twocolumn,groupedaddress]{revtex4}

% You should use BibTeX and apsrev.bst for references
% Choosing a journal automatically selects the correct APS
% BibTeX style file (bst file), so only uncomment the line
% below if necessary.
%\bibliographystyle{apsrev}
\usepackage{graphicx}
\usepackage{epstopdf}
\usepackage{color}
\usepackage{hyperref}
\hypersetup{colorlinks=true,linkcolor=blue,citecolor=blue,filecolor=blue,urlcolor=blue}
\definecolor{orange}{RGB}{255,127,0}
\definecolor{blue2}{RGB}{33,114,173}
%%%%%%%%%% Prefix a "S" to all equations, figures, tables and reset the counter %%%%%%%%%%
\setcounter{section}{0}
\setcounter{equation}{0}
\setcounter{figure}{0}
\setcounter{table}{0}
\setcounter{page}{1}
\makeatletter

\makeatother
%%%%%%%%%% Prefix a "S" to all equations, figures, tables and reset the counter %%%%%%%%%%

\begin{document}
%Title of paper
\title{Supplemental Material for:\\Electric Current Control of Helimagnetic Chirality from a Multidomain State in the helimagnet MnAu$_2$}
% \thanks{A footnote to the article title}%

\author{Yuta~Kimoto}
\affiliation{Institute for Materials Research, Tohoku University, Sendai 980-8577, Japan}
\author{Hidetoshi~Masuda}
\email{hidetoshi.masuda.c8@tohoku.ac.jp}
\affiliation{Institute for Materials Research, Tohoku University, Sendai 980-8577, Japan}
\author{Jun-ichiro~Ohe}
\affiliation{Department of Physics, Toho University, Funabashi 274-8510, Japan}
\author{Shoya~Sakamoto}
\affiliation{Institute for Materials Research, Tohoku University, Sendai 980-8577, Japan}
\affiliation{Center for Science and Innovation in Spintronics (CSIS), Core Research Cluster, Tohoku University, Sendai 980-8577, Japan}
\author{Takeshi~Seki}
\affiliation{Institute for Materials Research, Tohoku University, Sendai 980-8577, Japan}
\affiliation{Center for Science and Innovation in Spintronics (CSIS), Core Research Cluster, Tohoku University, Sendai 980-8577, Japan}
\author{Yoshinori~Onose}
\affiliation{Institute for Materials Research, Tohoku University, Sendai 980-8577, Japan}
\affiliation{Center for Science and Innovation in Spintronics (CSIS), Core Research Cluster, Tohoku University, Sendai 980-8577, Japan}

\maketitle
%\tableofcontents
\newpage

\section{Differential resistivity}
Fig. S1 exhibits the differential resistivity subtracted by a quadratic background $\rho_0\alpha j_\mathrm{dc}^2$ at various magnetic fields at 250 K. Here, $\rho_0$ and $j_\mathrm{dc}$ are linear resistivity and bias dc electric current, respectively, and $\alpha =1.40\times 10^{-15}$ A$^{-2}$m$^4$.
The sample measured in this work is identical to sample $\#2$ shown in the Supplemental Material of ref. \cite{kimoto} and Fig. S1 is reproduced from ref. \cite{kimoto}. 
The differential resistivity shows kinks at the threshold electric currents of sliding indicated by arrows between 1.5 T and 2.25 T. In the magnetic field region, we observed the field-symmetric peaks in the magnetic field dependence of $\rho^{2\omega}$ (see Figs. 1(d) and (f) in the main text). Since $\rho^{2\omega}$ was measured using ac current with an amplitude of $4.2\times 10^9$ A/m$^2$, which exceeds the threshold currents, the origin of peaks in $\rho^{2\omega}$ seems to be the kinks in the differential resistivity due to the sliding motion.

\begin{figure}[ht]
  \includegraphics[width=7cm]{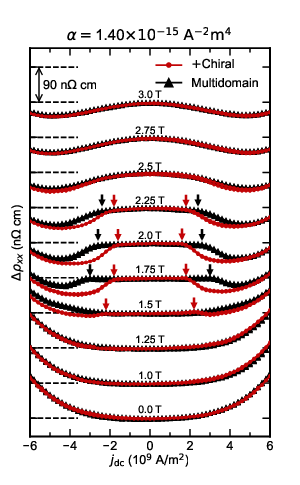}
  \caption{The differential resistivity subtracted by a quadratic background as a function of bias dc current $j_\mathrm{dc}$ at various magnetic fields at 250 K.}
  \label{FigS2}
\end{figure}
\newpage

\section{Experimental data of $\rho^{2\omega}$ at respective temperatures}
In the main text, the experimental data at 250 K are shown. We here present the experimental data at 300 K, 275 K, 225 K, and 200 K. We could not measure the data below 200 K because of small magnitude of $\rho^{2\omega}$.

\subsection{300 K}
We show the magnetic field dependence of $\rho^{2\omega}$ at 300 K and the antisymmetric and symmetric components in Fig. S2. These correspond to Figs. 1(d)-(f) in the main text. In Fig. S3, we show the variation of $\rho^{2\omega}$ after the application of an electric current pulse at various magnetic fields at 300 K. This corresponds to Fig. 3 in the main text, and the measurement conditions are identical, except that an ac current with an amplitude of $2.1 \times 10^9~\mathrm{A/m^2}$ was used. The transition from the multidomain state to a single-chiral domain state was not observed in the low-field region.

\begin{figure}[ht]
  \includegraphics[width=9cm]{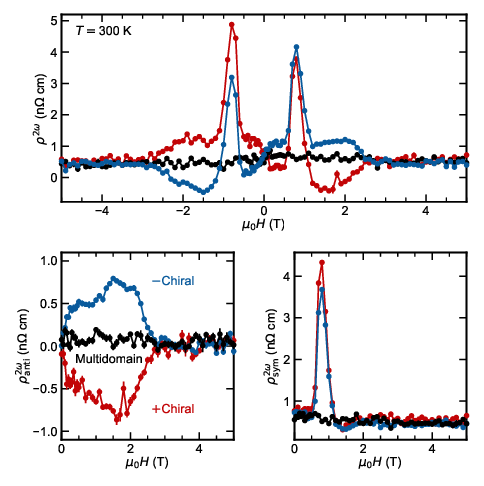}
  \caption{(a) Second-harmonic resistivity $\rho^{2\omega}$ as a function of magnetic field at 300 K. Before the measurements, as detailed in the main text, $+$Chiral, $-$Chiral, and multidomain states were prepared by the magnetic field sweep from $+$5 T to 0 T with positive and negative currents and without current, respectively. The data in the positive magnetic field region was obtained by increasing the magnetic field from the controlled initial states at 0 T, whereas the data in the negative magnetic field region was obtained by decreasing the magnetic field from the separately prepared initial states. (e) The field-antisymmetric component of second-harmonic resistivity $\rho^{2\omega}_\mathrm{anti}=(\rho^{2\omega}(+H)-\rho^{2\omega}(-H))/2$. (f) The field-symmetric component of second-harmonic resistivity $\rho^{2\omega}_\mathrm{sym}=(\rho^{2\omega}(+H)+\rho^{2\omega}(-H))/2$.}
  \label{FigS_300K_rho2f}
\end{figure}

\begin{figure}[ht]
  \includegraphics{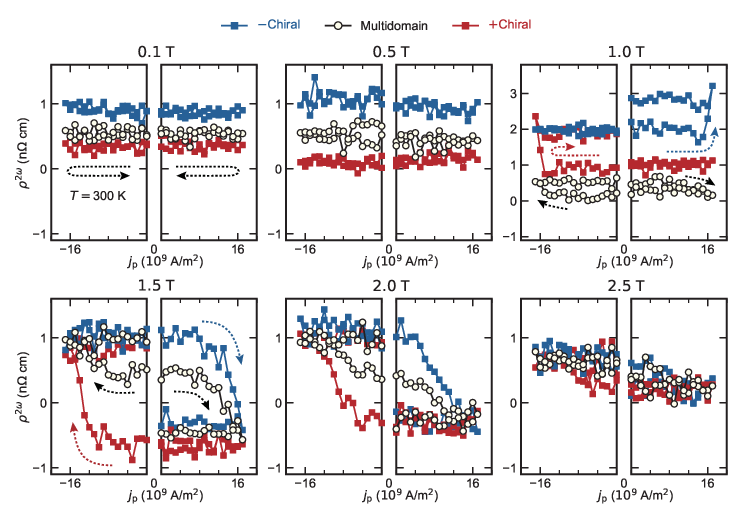}
  \caption{Second-harmonic resistivity $\rho^{2\omega}$ measured after the application of an electric current pulse $j_\mathrm{p}$ at various magnetic fields at 300 K. The electric current pulses were repeatedly applied with changing the magnitude as shown by dotted arrows, and $\rho^{2\omega}$ was measured after each current pulse application. For each field, two subfigures are shown in this figure: in the left subfigure, the electric current was decreased from 0 A/m$^2$ to $-17\times 10^9$ A/m$^2$ and then increased back to 0 A/m$^2$; in the right subfigure, it was increased from 0 A/m$^2$ to $+17\times 10^9$ A/m$^2$ and subsequently decreased back to 0 A/m$^2$. The initial $+$Chiral, $-$Chiral, and multidomain states were prepared similarly to the main text. Note that the range of the vertical axis is larger at 1.0 T.}
  \label{FigS_300K_control}
\end{figure}
\clearpage

\subsection{275 K}
We show the magnetic field dependence of $\rho^{2\omega}$ and the antisymmetric and symmetric components at 275 K in Fig. S4. We also show the variation of $\rho^{2\omega}$ after the application of an electric current pulse at various magnetic fields at 275 K in Fig. S5. The measurements were performed using an ac current with an amplitude of $4.2\times 10^9$ A/m$^2$. The transition from the multidomain state to a single-chiral domain state was barely observed at 0.5 T. 

\begin{figure}[ht]
  \includegraphics[width=9cm]{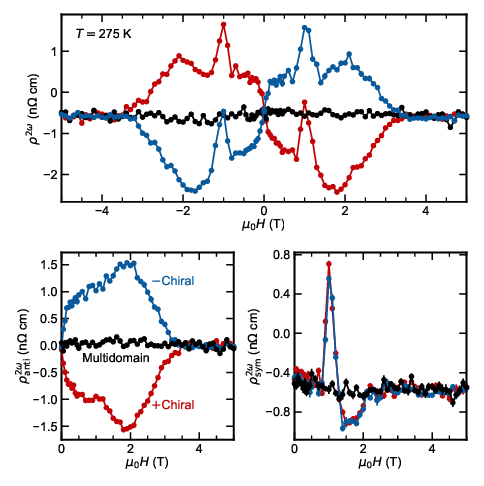}
  \caption{(a) Second-harmonic resistivity $\rho^{2\omega}$ as a function of magnetic fields at 275 K. Before the measurements, as detailed in the main text, $+$Chiral, $-$Chiral, and multidomain states were prepared by the magnetic field sweep from $+$5 T to 0 T with positive and negative currents and without current, respectively. The data in the positive magnetic field region was obtained by increasing the magnetic field from the controlled initial states at 0 T, whereas the data in the negative magnetic field region was obtained by decreasing the magnetic field from the separately prepared initial states. (e) The field-antisymmetric component of second-harmonic resistivity $\rho^{2\omega}_\mathrm{anti}=(\rho^{2\omega}(+H)-\rho^{2\omega}(-H))/2$. (f) The field-symmetric component of second-harmonic resistivity $\rho^{2\omega}_\mathrm{sym}=(\rho^{2\omega}(+H)+\rho^{2\omega}(-H))/2$.}
  \label{FigS_275K_rho2f}
\end{figure}
\begin{figure}[ht]
  \includegraphics{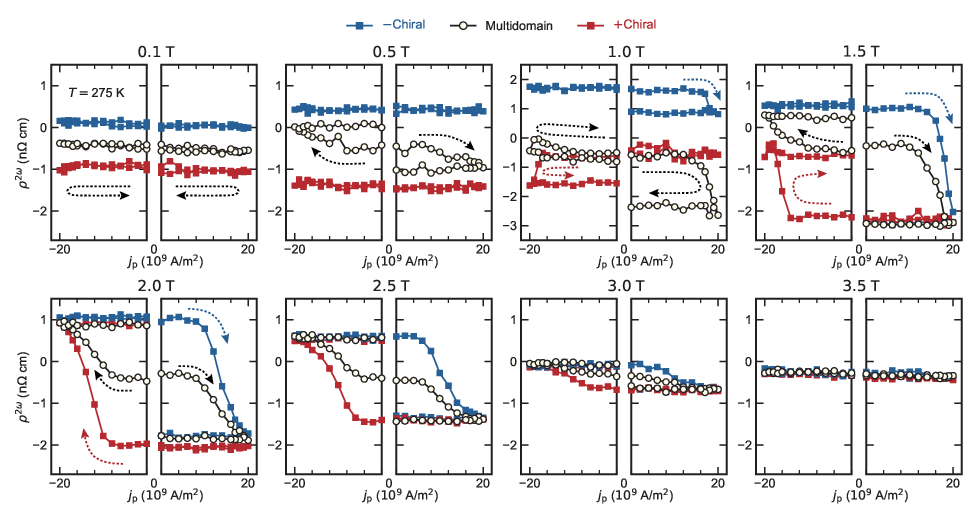}
  \caption{Second-harmonic resistivity $\rho^{2\omega}$ measured after the application of an electric current pulse $j_\mathrm{p}$ at various magnetic fields at 275 K. The electric current pulses were repeatedly applied with changing the magnitude as shown by dotted arrows, and $\rho^{2\omega}$ was measured after each current pulse application. For each field, two subfigures are shown in this figure: in the left subfigure, the electric current was decreased from 0 A/m$^2$ to $-20\times 10^9$ A/m$^2$ and then increased back to 0 A/m$^2$; in the right subfigure, it was increased from 0 A/m$^2$ to $+20\times 10^9$ A/m$^2$ and subsequently decreased back to 0 A/m$^2$. The initial $+$Chiral, $-$Chiral, and multidomain states were prepared similarly to the main text. Note that the range of the vertical axis is larger at 1.0 T.}
  \label{FigS_275K_control}
\end{figure}
\clearpage

\subsection{225 K}
Similarly to the cases of 300 K and 275 K, we show the magnetic field dependence of $\rho^{2\omega}$ and the antisymmetric and symmetric components at 225 K in Fig. S6, and the variation of $\rho^{2\omega}$ after the application of an electric current pulse at various magnetic fields at 225 K in Fig. S7. The measurements were performed using an ac current with an amplitude of $6.4\times 10^9$ A/m$^2$. The transition from the multidomain state to a single-chiral domain state was observed in the low-field region, similar to 250 K. In addition, the chirality reversal from a uniform chiral state was also observed at 0.1 T, but with a higher threshold current.

\begin{figure}[ht]
  \includegraphics[width=9cm]{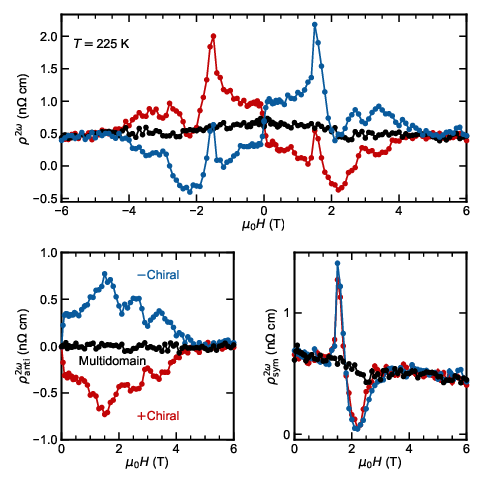}
  \caption{(a) Second-harmonic resistivity $\rho^{2\omega}$ as a function of magnetic field at 225 K. Before the measurements, as detailed in the main text, $+$Chiral, $-$Chiral, and multidomain states were prepared by the magnetic field sweep from $+$5 T to 0 T with positive and negative currents and without current, respectively. The data in the positive magnetic field region was obtained by increasing the magnetic field from the controlled initial states at 0 T, whereas the data in the negative magnetic field region was obtained by decreasing the magnetic field from the separately prepared initial states. (e) The field-antisymmetric component of second-harmonic resistivity $\rho^{2\omega}_\mathrm{anti}=(\rho^{2\omega}(+H)-\rho^{2\omega}(-H))/2$. (f) The field-symmetric component of second-harmonic resistivity $\rho^{2\omega}_\mathrm{sym}=(\rho^{2\omega}(+H)+\rho^{2\omega}(-H))/2$.}
  \label{FigS_225K_rho2f}
\end{figure}
\begin{figure}[ht]
  \includegraphics{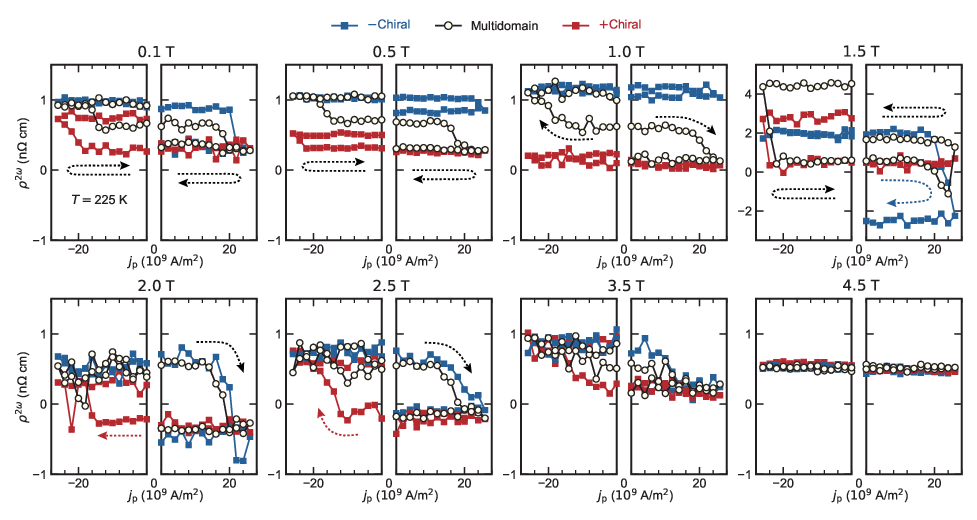}
  \caption{Second-harmonic resistivity $\rho^{2\omega}$ measured after the application of an electric current pulse $j_\mathrm{p}$ at various magnetic fields at 225 K. The electric current pulses were repeatedly applied with changing the magnitude as shown by dotted arrows, and $\rho^{2\omega}$ was measured after each current pulse application. For each field, two subfigures are shown in this figure: in the left subfigure, the electric current was decreased from 0 A/m$^2$ to $-26\times 10^9$ A/m$^2$ and then increased back to 0 A/m$^2$; in the right subfigure, it was increased from 0 A/m$^2$ to $+26\times 10^9$ A/m$^2$ and subsequently decreased back to 0 A/m$^2$. The initial $+$Chiral, $-$Chiral, and multidomain states were prepared similarly to the main text. Note that the range of the vertical axis is larger at 1.5 T.}
  \label{FigS_225K_control}
\end{figure}
\clearpage

\subsection{200 K}
Similarly, we show the magnetic field dependence of $\rho^{2\omega}$ and the antisymmetric and symmetric components at 200 K in Fig. S8, and the variation of $\rho^{2\omega}$ after the application of an electric current pulse at various magnetic fields at 200 K in Fig. S9. The measurements were performed using an ac current with an amplitude of $6.4\times 10^9$ A/m$^2$. The chirality reversal from a uniform chiral state was also observed in the low-field region. Because the threshold current increases with increasing magnetic field, the low-field reversal phenomenon cannot be attributed to the effect of Joule heating. The non-thermal chirality reversal in the low-field and low-temperature region is also very interesting and might be useful for future application, but we could not pursue further at present because $\rho^{2\omega}$ is very small in this temperature region.

\begin{figure}[ht]
  \includegraphics[width=9cm]{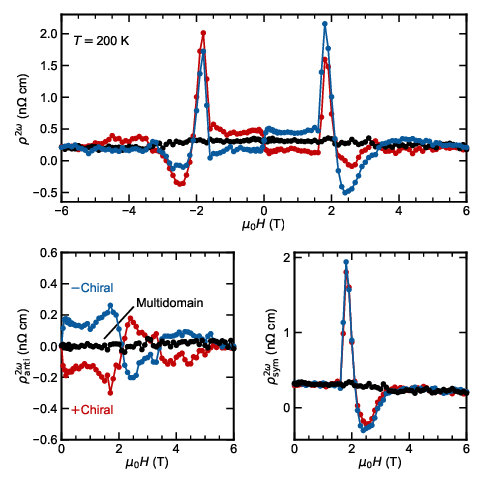}
  \caption{(a) Second-harmonic resistivity $\rho^{2\omega}$ as a function of magnetic field at 200 K. Before the measurements, as detailed in the main text, $+$Chiral, $-$Chiral, and multidomain states were prepared by the magnetic field sweep from $+$5 T to 0 T with positive and negative currents and without current, respectively. The data in the positive magnetic field region was obtained by increasing the magnetic field from the controlled initial states at 0 T, whereas the data in the negative magnetic field region was obtained by decreasing the magnetic field from the separately prepared initial states. (e) The field-antisymmetric component of second-harmonic resistivity $\rho^{2\omega}_\mathrm{anti}=(\rho^{2\omega}(+H)-\rho^{2\omega}(-H))/2$. (f) The field-symmetric component of second-harmonic resistivity $\rho^{2\omega}_\mathrm{sym}=(\rho^{2\omega}(+H)+\rho^{2\omega}(-H))/2$.}
  \label{FigS_200K_rho2f}
\end{figure}
\begin{figure}[ht]
  \includegraphics{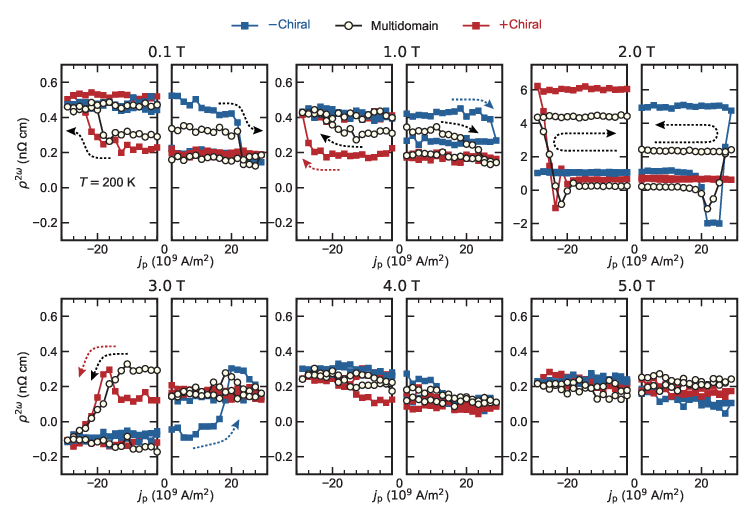}
  \caption{Second-harmonic resistivity $\rho^{2\omega}$ measured after the application of an electric current pulse $j_\mathrm{p}$ at various magnetic fields at 200 K. The electric current pulses were repeatedly applied with changing the magnitude as shown by dotted arrows, and $\rho^{2\omega}$ was measured after each current pulse application. For each field, two subfigures are shown in this figure: in the left subfigure, the electric current was decreased from 0 A/m$^2$ to $-30\times 10^9$ A/m$^2$ and then increased back to 0mA; in the right subfigure, it was increased from 0 A/m$^2$ to $+30\times 10^9$ A/m$^2$ and subsequently
decreased back to 0 A/m$^2$. The initial $+$Chiral, $-$Chiral, and multidomain states were prepared similarly to the main text. Note that the range of the vertical axis is larger at 2.0 T.}
  \label{FigS_200K_control}
\end{figure}
\newpage

% \bibliography{Supple}% Produces the bibliography via BibTeX.

\end{document}
